# Supplementary material for: Constraining new physics with a novel measurement of the $^{23}$Ne $\beta$-decay branching ratio
Source: arXiv:2107.14355 ancillary file (2021-07-29)
Supplement: Supplementary file 1 [file Supp.pdf]

# Supplemental Material: Constraining new physics with a novel measurement of the $^{23}$Ne $\beta$-decay branching ratio

Yonatan Mishnayot[a,b], Ayala Glick-Magid[a], Hitesh Rahangdale[a], Guy Ron [a,*], Doron Gazit[a], Jason T. Harke[c], Michael Hass[d,1], Ben Ohayon[a,e], Aaron Gallant[c], Nicholas D. Scielzo[c], Sergey Vaintraub[b], Richard O. Hughes[c], Tsviki Hirsh[b], Christian Forssén[f], Daniel Gazda[g], Peter Gysbers[h,i], Javier Menéndez[j], Petr Navrátil[h], Leonid Weissman[b], Arik Kreisel[b], Boaz Kaizer[b], Hodaya Dafna[b], Maayan Buzaglo[b]

[a]*The Racah Institute of Physics, The Hebrew University of Jerusalem, Givat Ram, Jerusalem, 9190401*

[b]*Soreq Nuclear Research Center, Yavne, 8180000*

[c]*Lawrence Livermore National Laboratory, Livermore, CA, USA*

[d]*Department of Particle Physics, Weizamnn Institute of Science, Rehovot, Israel*

[e]*Institute for Particle Physics and Astrophysics, ETH Zürich, CH-8093 Zürich, Switzerland*

[f]*Department of Physics, Chalmers University of Technology, SE-412 96 Göteborg, Sweden*

[g]*Nuclear Physics Institute, 25068 Řež, Czech Republic*

[h]*TRIUMF, 4004 Wesbrook Mall, Vancouver, British Columbia V6T 2A3, Canada*

[i]*Department of Physics and Astronomy, University of British Columbia, Vancouver, British Columbia, Canada*

[j]*Department of Quantum Physics and Astrophysics and Institute of Cosmos Sciences, University of Barcelona, 08028 Barcelona, Spain*

---

## Contents

**1 $^{23}$Ne production 2**

*Corresponding author
*Email address:* `guy.ron2@mail.huji.ac.il` ( Guy Ron )

[1]Deceased.

**2 Detector Calibration** **5**
2.1 $\gamma$ Spectrum . . . . . 5
2.2 HPGe Energy Calibration . . . . . 5
2.3 HPGe Detector Efficiency Calibration . . . . . 6
2.4 $\beta$ detector energy calibration . . . . . 6

**3 Corrections** **11**
3.1 $N_\beta$ . . . . . 11
3.1.1 Events outside the measurement cell . . . . . 11
3.1.2 Random coincidences . . . . . 11
3.1.3 Contaminants . . . . . 11
3.1.4 $N_\beta$ summary . . . . . 12
3.2 $N_{\beta\gamma}$ . . . . . 12
3.2.1 $\beta$ detector threshold . . . . . 12
3.2.2 Higher state contributions . . . . . 13
3.2.3 Deadtime correction . . . . . 14
3.2.4 Random Coincidence . . . . . 15
3.2.5 $N_{\beta\gamma}$ Corrections - Summary . . . . . 15
3.3 $\varepsilon_\gamma$ - Volume correction . . . . . 15

**4 Extraction of the branching ratio** **17**

**5 Validation - $^6$He** **21**

**6 Explicit expressions of the multipole operators** **22**

**7 Nuclear matrix elements for the $\beta$ decay of $^{23}$Ne** **23**

## 1. $^{23}$Ne production

$^{23}$Ne was produced via the (n,p) reaction on the $^{23}$Na content in natural abundance NaCl. Neutrons were produced in the SARAF facility using the (d,n) reaction in a liquid-lithium target [1, 2, 3, 4, 5]. To increase the yield the NaCl was finely milled to an average crystal size of approximately 40 $\mu$m and heated to 600 °C. A vacuum chamber containing the milled, heated, salt, was placed in front of the neutron production target (Fig. 1) and connected via a low-pressure transport vacuum line backed by a turbomolecular pump whose output was directed to a cold trap, used to remove contaminants and then connected to the measurement cell. Fig. 2 shows a schematic of the vacuum

and transport system connecting the production target to the measurement cell, the radioactive atoms were transported via diffusion to the measurement cell which was continuously pumped on by a scroll pump to maintain a steady flow rate of fresh neon-23 in the measurement cell. A complete description of the production setup may be found in [6].

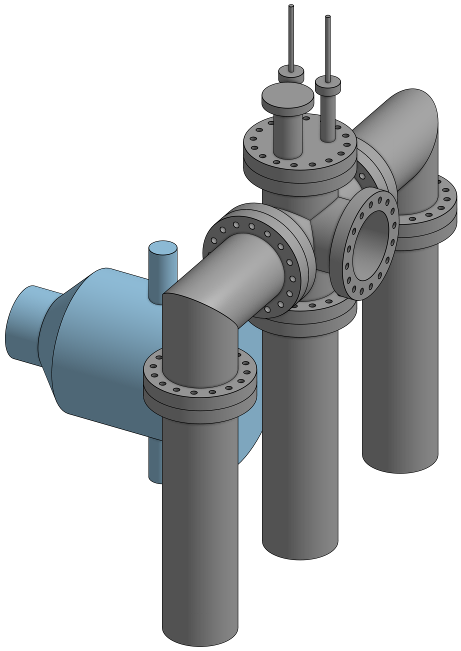

Figure 1: A schematic of the $^{23}$Ne production target (NaCl cell, in gray) next to the neutron (liquid lithium) production target (in teal).

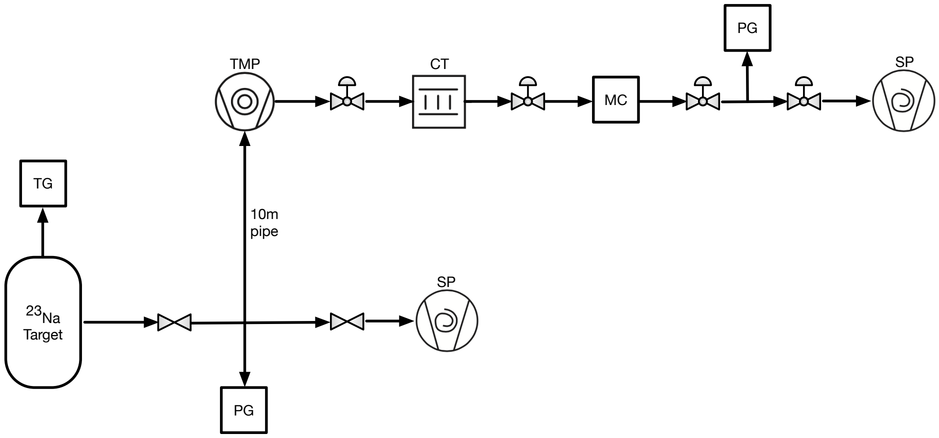


Figure 2: A schematic sketch of the experimental system, a 4-inch diameter, 5 meter length hose connects the $^{23}$Na target to a valve. Another 4-inch, 10 meter length pipe transports the gas from the target room to the turbo pump. From the turbo pump, plastic hoses of 6 mm diameter connect the different elements. TG denotes a temperature gauge, PG denotes a pressure gauge, MC denotes the measurement cell, TMP denotes a turbomolecular pump, SC denotes a scroll pump, a CT denotes a cold trap.

## 2. Detector Calibration

### *2.1. $\gamma$ Spectrum*

As an indication of the quality of the data Fig. 3 show the $\gamma$ spectrum near the 440 keV line as measured using the HPGe detector, with and without coincidence with the $\beta$ particle detected with the scintillators. The quality of the data, as well as the reduction of the background, is evident.

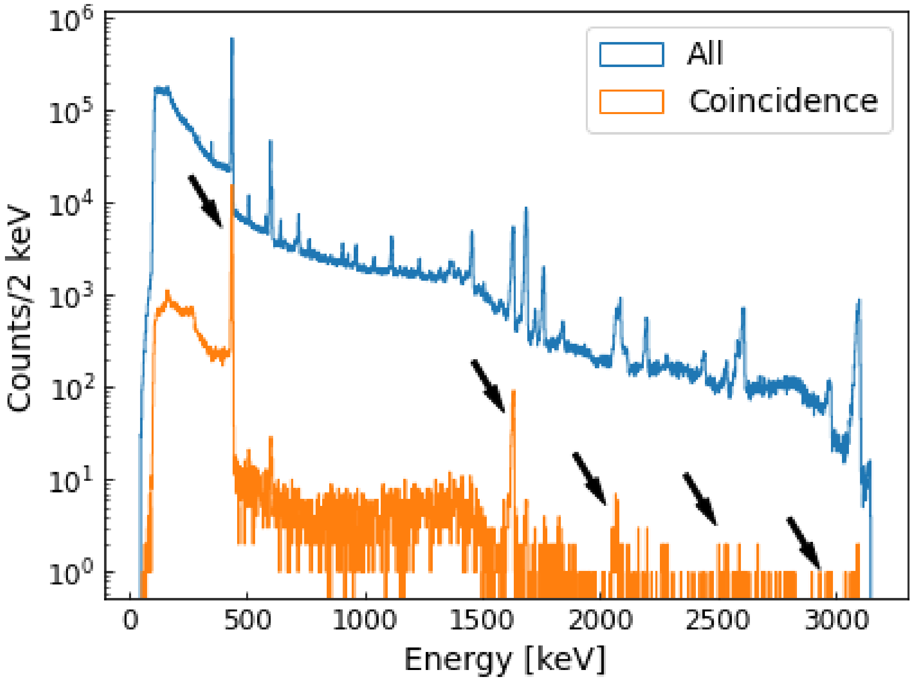


Figure 3: The $\gamma$ spectrum (at 16 cm distance) as measured with the HPGe detector, with (orange) and without (blue) coincidence with the $\beta$ detectors, the $^{23}$Ne peaks at 440, 1636, 2076, 2542, and 2982 keV are marked with black arrows, the rightmost peak is the $^{37}$S background.

### *2.2. HPGe Energy Calibration*

The HPGe detector energy was calibrated with a set of calibrated radionuclides using a linear fit to map channel to $\gamma$ energy, for the list of sources see below (2.3).

*2.3. HPGe Detector Efficiency Calibration*

To reduce systematic effects, the measurements were taken with the HPGe detector at two distances relative to the face of the measurement cell (16 cm, and 20 cm). For each of those distances, the HPGe detector efficiency was determined at the two relevant energies (440 and 1636 keV) using a set of calibrated sources spanning a wide energy range. For each of the sources, the photopeak was calculated by fitting the peak shape to an exponentially modified Gaussian on top of a smoothed step function and a linear background, the results of the fit were used to determine the number of events in the photopeak, which together with the known source activity provides the HPGe efficiency at the photopeak energy.

The radio-nuclides used had $\gamma$ energies in the range of 122–1836 keV: $^{57}$Co, $^{133}$Ba, $^{137}$Cs, $^{54}$Mn, $^{88}$Y, $^{Co}$60 and $^{22}$Na. Except for $^{22}$Na, all sources are of EG3 type with an uncertainty lower than 1%, manufactured by CMI. The $^{22}$Na source was manufactured by Eckert & Ziegler with a one sigma uncertainty of 1.5%. In addition, we used a multi-source manufactured by Eckert & Ziegler from NG-2 solution with $\gamma$ energies in the range 88–1836 keV, which includes $^{109}$Cd, $^{57}$Co, $^{139}$Ce, $^{202}$Hg, $^{119}$Sn, $^{85}$Sr, $^{137}$Cs, $^{88}$Y and $^{60}$Co. The multi-source one sigma uncertainties were 1.5% except for $^{109}$Cd which had a $1\sigma$ uncertainty of 2.5%. Table 1 lists the sources, $\gamma$-energies, and the uncertainties on the source activity use in the calibration.

The measured efficiencies were used to determine the HPGe efficiency at 440 and 1636 keV using the function:

$$\varepsilon(E_\gamma) = \frac{1}{P_1 E_\gamma^{P_2} + P_3 E_\gamma^{P_4}}, \tag{1}$$

where $\varepsilon$ is the detector efficiency, $E_\gamma$ is the photon energy, and $P_i$ are fit parameters. Fig. 4 shows the result of the fit for the various detector positions. The uncertainties on efficiencies for the 440 and 1636 keV lines were scaled by $\sqrt{\chi_\nu}$ to obtain a more conservative estimate of the photopeak efficiency uncertainty.

*2.4. $\beta$ detector energy calibration*

In order to apply threshold corrections on the measurement, one must calibrate the thick scintillator detector energy.

To determine both the energy calibration and resolution, $\gamma$-ray sources were used. Here, the $\gamma$-ray Compton edges are used to find both the energy and the resolution at a given energy.

| Isotope | $\gamma$ energy [keV] | Uncertainty on the activity [%] |
|---|---|---|
| $^{109}$Cd | 88 | 2.5 |
| $^{57}$Co | 122 | 1.5 |
| $^{57}$Co | 122 | 0.5 |
| $^{139}$Ce | 166 | 1.5 |
| $^{133}$Ba | 276 | 0.7 |
| $^{203}$Hg | 279 | 1.5 |
| $^{133}$Ba | 303 | 0.7 |
| $^{133}$Ba | 356 | 0.7 |
| $^{133}$Ba | 384 | 0.7 |
| $^{113}$Sn | 392 | 1.5 |
| $^{137}$Cs | 662 | 1.5 |
| $^{137}$Cs | 662 | 0.8 |
| $^{54}$Mn | 835 | 0.5 |
| $^{88}$Y | 898 | 1.5 |
| $^{88}$Y | 898 | 0.6 |
| $^{60}$Co | 1173 | 1.5 |
| $^{60}$Co | 1173 | 0.6 |
| 22Na | 1275 | 1.5 |
| $^{60}$Co | 1332 | 0.6 |
| $^{88}$Y | 1836 | 1.5 |
| $^{88}$Y | 1836 | 0.6 |

Table 1: The sources used in the calibration of the HPGe detector efficiency

Here we follow a method suggested by Safari et al. [7], they suggest a mathematical description of the Compton edge behavior in a plastic scintillator – the response function – as a convolution of an ideal response function with a Gaussian peak. Using this method, one can fit the experimental data to a mathematical description and extract both Compton edge and energy resolution without resorting to simulations.

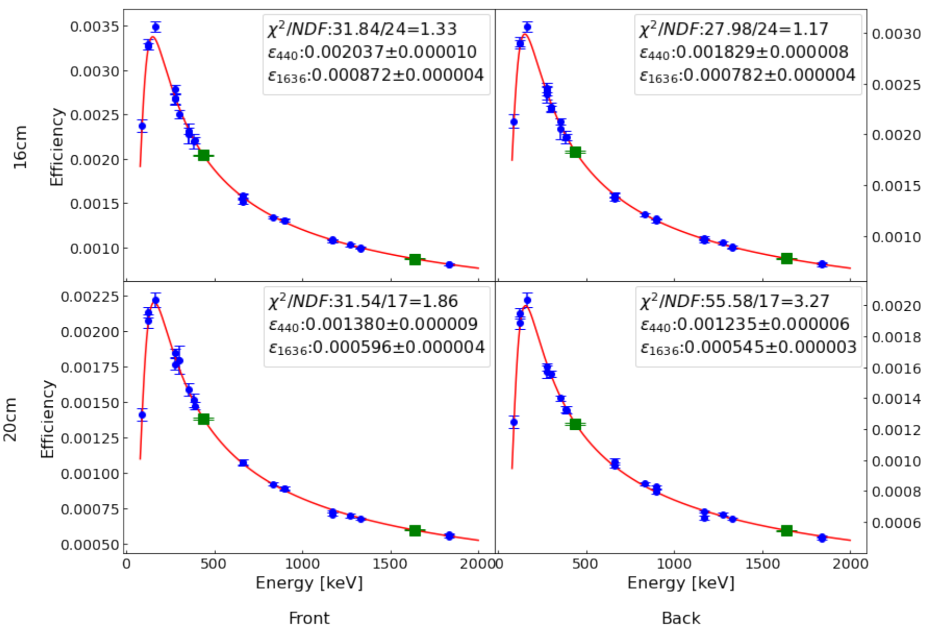


Figure 4: The fit for the HPGe detector efficiency for the detector positions used in the experiment.

The response function is:

$$
\begin{aligned}
R(E) &= \alpha(E) \cdot \text{erfc}[\frac{E - E_C}{\sqrt{2}\sigma}] + \beta(E) \cdot \exp[-\frac{(E - E_C)^2}{2\sigma^2}] \\
\alpha(E) &= \frac{1}{2}[a(E^2 + \sigma^2) + bE + c] \\
\beta(E) &= \frac{-\sigma}{\sqrt{2\pi}} a(E + E_C) + b
\end{aligned}
\quad (2)
$$

where E denotes the energy, $E_C$ denotes the Compton edge energy, and $\sigma$ denotes the variance. The constants a, b and c are derived from the theoretical response function:

$$
r(E) = \begin{cases} aE^2 + bE + c & E \leq E_C \\ 0 & E > E_C \end{cases} \quad (3)
$$

fitting the experimental data to Eq. 2 allows one to find both $E_C$ and $\sigma$. The resolution is given by [8]:

$$
\epsilon_\beta = 2\sqrt{2\ln 2}\frac{\sigma}{E_C} \quad (4)
$$

Evaluating the resolution at several points using Eq. 4, one can fit the resolution to a power model law to get the resolution over the whole energy range:

$$\epsilon_\beta = \alpha E^\beta \tag{5}$$

The calibration of the thick plastic scintillator was performed using the Compton edges of the following sources: $^{57}$Co, $^{133}$Ba, $^{22}$Na, $^{207}$Bi, $^{54}$Mn and $^{88}$Y. In addition, the $^{207}$Bi K shell conversion electron peak (CE K) was used to verify the calibration process.

The different Compton edges were fit with Eq. 2 extracting both Compton edge (channel) and its variance (See e.g. Fig. 5). The Compton energy was calculated for the back scattering angle in the Compton scattering equation [8]. Having the Compton edge and its variance, a linear fit was used to find the calibration, and Eq. 4 was used to determine the resolution.

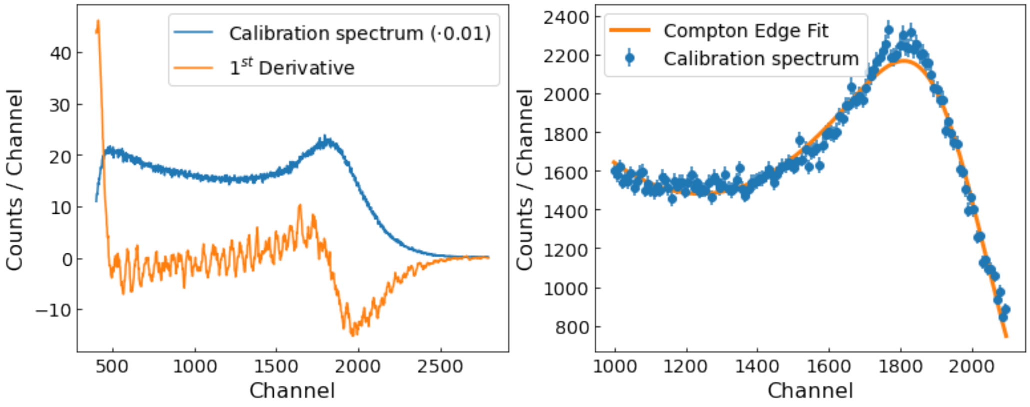


Figure 5: Left: $^{137}$Cs spectrum and its derivative. Right: Zoom in on the Compton edge and the fit.

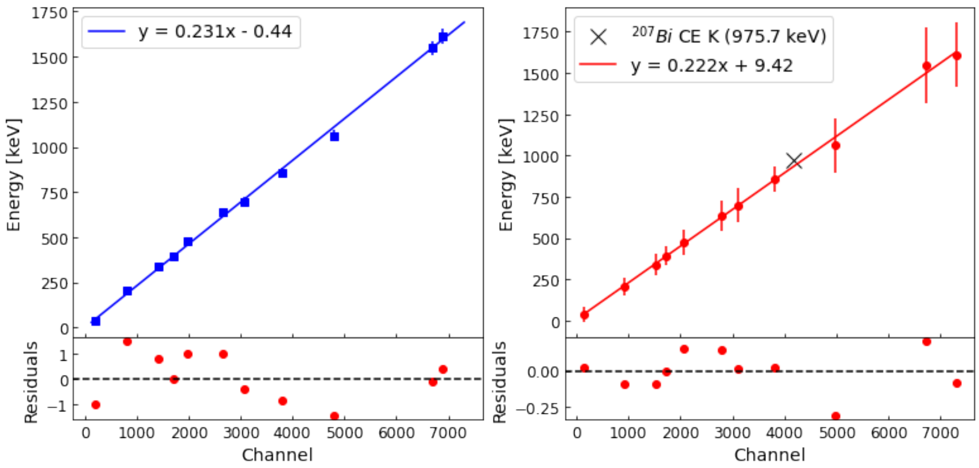


Figure 6: Thick scintillator energy calibration. Left – Compton edges defined by the derivative minimum. Right – Compton edges defined by fit, the black X denotes the $^{207}$Bi conversion electron that was used as a cross-check.

## 3. Corrections

The branching ratio is calculated as:

$$BR_{440keV} = \frac{\mathrm{N}_{\beta\gamma}}{\epsilon_\gamma \mathrm{N}_\beta}. \quad (6)$$

Several corrections must be applied to the number of measured $\beta$ events and to the number of $\beta - \gamma$ coincidence events. Here we list the corrections that were applied.

### *3.1. $N_\beta$*

#### *3.1.1. Events outside the measurement cell*

To estimate the number of $\beta$ particles that originated outside the measurement cell, background runs were taken in which thick tantalum foil was placed between the scintillators and the measurement cell. The number of detected $\beta$ particles from these runs were used to estimate the background originating from outside the measurement cell, which is then subtracted from the data.

#### *3.1.2. Random coincidences*

To estimate the random coincidences, the random region of the time difference spectrum between the thick and thin detector was used to determine the background under the prompt peak. The number of random coincidences was then subtracted from the data. Since the coincidence peak was several orders of magnitude above the background, its upper limit is 0.14% for all runs.

#### *3.1.3. Contaminants*

Radioactive contaminants that were transported inside the vacuum transport line were removed using a cold trap situated between the production target and the measurement cell. The cold trap was cooled with liquid nitrogen. However, during the measurements, besides the 440 keV and 1636 keV peaks, the 3103 keV peak from $^{37}$S was detected . The $^{37}$S was produced via the $^{37}$Cl(n,p)$^{37}$S reaction within the salt target, and has a relatively short half-life of 5.05 m. The upper limit for its contribution to the $\beta$ spectrum was evaluated to be 0.06% for all runs.

In contrast to the energy resolution 1-2 keV for the HPGe detector, the plastic scintillator detector resolution is quite poor ($\approx$ 20%). Any $\beta$ decaying

isotope can contribute to the $\beta$ spectrum ($N_\beta$) and thus decrease the BR artificially. A good estimate of the contaminant contributions is needed to correct $N_\beta$ to obtain the $^{23}$Ne BR properly. To estimate the amount of contamination present in the measurement cell, $\beta$-$\gamma$-ray coincidence events were used. While the $\beta$ spectrum is continuous, the individual $\gamma$-rays from a contaminant $\beta$-particle emitting isotope are unique and can be identified using the HPGe detector. Contaminant isotopes were identified in the $\gamma$-ray spectrum, and the corresponding $\beta$-particle spectrum was determined by looking at the $\beta$-$\gamma$-ray coincidence with the unique $\gamma$-ray. In this way, the relative contribution of the contaminants to the $\beta$ spectrum were estimated by comparing it to the number of $\beta$ events extracted from the 440 keV peak from $^{23}$Ne. To extract the contaminant contribution to the $\beta$ spectrum, its relative contribution to the $\beta$-$\gamma$-ray coincidence spectrum was used as follows:

$$k_{cont} = (\frac{N_{3103\beta\gamma}}{\epsilon_{3103}} \cdot \frac{\epsilon_{440}}{N_{\beta\gamma}})\frac{N_{\beta\gamma}}{\epsilon_{440} \cdot BR_1} \tag{7}$$

where $N_{3103\beta\gamma}$, $N_{\beta\gamma}$ denotes the contaminant and the $^{23}$Ne 440 keV peak contributions to the $\beta$-$\gamma$-ray coincidence spectrum, respectively. $\epsilon_{3103}$, $\epsilon_{440}$ denotes the efficiencies at the relevant energies in keV, respectively. Finally, $BR_1$ represents the BR of the $1^{st}$ excited state of $^{23}$Na.

#### *3.1.4. $N_\beta$ summary*

Summarizing the $N_\beta$ corrections, the term for the net number of $\beta$ events is written as:

$$N_\beta = (N_\beta^m - N_{bgd} - N_{rand}) \cdot k_{cont} \tag{8}$$

where $N_\beta$ denotes the net number of $\beta$-particles, $N_\beta^m$ denotes the number of $\beta$ measured events respectively. $N_{bgd}$, $N_{rand}$ denotes the background and random coincidence terms as detailed above, respectively, and $k_{cont}$ denotes the contaminant correction.

### *3.2. $N_{\beta\gamma}$*

#### *3.2.1. $\beta$ detector threshold*

Since the endpoint energy of the $\beta$ particle spectrum is different in the decays to the ground and excited states of $^{23}$Na, the effect of the scintillator detector threshold must be taken into account.

As the $\beta$-particle detector threshold increases, less 440 keV $\gamma$-ray events in coincidence with $\beta$ particles would be measured than expected. This correction for this effect was determined using a GEANT4 [9, 10, 11] simulation as follows:

1. The $\beta$-particle spectrum of each state was determined analytically using a $\beta$ Spectrum Generator [12].
2. The $\beta$ spectrum for each final state was fed into a GEANT4 simulation of the system, which included the measurement cell and plastic scintillator detectors.
3. The GEANT4 simulation was used to determine the $\beta$ spectrum measured by the thick scintillator.
4. The simulated $\beta$ spectrum was used to evaluate the correction.

With the simulated $\beta$ spectrum, the correction is expressed as follows:

$$\begin{aligned} b_i(T) &= \frac{\int_T^{E_0} \frac{dN_e}{dW} dW}{\int_0^{E_0} \frac{dN_e}{dW} dW} \\ k_{thres} &= \left(\frac{b_1(T)}{\sum_{i=0}^{2} b_i(T)\eta_i}\right)^{-1} \end{aligned} \tag{9}$$

where $\int \frac{dN_e}{dW} dE$ denotes the integral of the differential $\beta$ spectrum over the energy range, $T$, $E_0$ denotes the threshold and Q-value, respectively. $b_i(T) \in (0, 1)$ denotes the fraction of spectrum above threshold for each state, and $\eta_i$ denotes the BR of the state i. Since the last excited state contribution is negligible, it was omitted from the evaluation of the threshold correction. Fig. 7 shows the threshold correction as a function of the actual detector threshold cut-off. For all the results discussed a threshold of 150 keV was used which corresponds to a correction of factor of 1.0012 to the $\beta$-particle spectrum.

*3.2.2. Higher state contributions*

The transition to the $3^{rd}$ excited state of $^{23}$Na has a low $\beta$-decay transition probability of 0.065%, therefore it can be neglected during the evaluation of the different $\beta$-spectrum corrections. As a result, the $\beta$-spectrum corrections only include the transition between the $2^{nd}$ excited state of $^{23}$Na to the $1^{st}$ excited state, with an energy of 1636 keV. Since the $\gamma$-ray branching ratio is known quite well, this correction can be applied either by using its relative

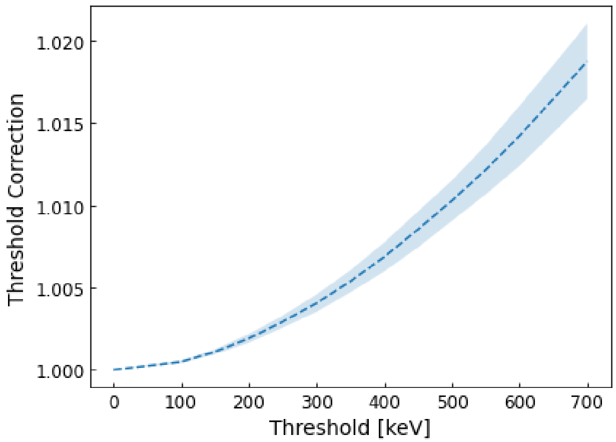


Figure 7: The $\beta$-spectrum threshold correction as a function of threshold cut-off energy, the filled band shows the $1\sigma$ uncertainty band.

intensity as extracted from [13] (3.03%) or by evaluating the contribution of that transition from within the experimental data. Here, the value of [13] was used, as follows:

$$N^c_{HS} = 1 - I_{1636} \tag{10}$$

where $I_{1636}$ denotes the intensity of the 1636 keV $\gamma$ relative to the 440 keV $\gamma$ - 0.0303.

*3.2.3. Deadtime correction*

To determine the data acquisition dead time, a 50 Hz pulser signal ($R_p$) was injected into the $\gamma$-ray spectrum via the test input cable on the HPGe detector. The pulser peak effective energy was set well above the main $\gamma$-ray spectrum, and was at $\approx$ 5.5 MeV. The dead-time is defined as the ratio between the pulser peak area in the $\gamma$-ray spectrum and the expected number of pulser events ($N_p$) for the measurement of time and is given by:

$$\begin{aligned} N_p =& R_p \cdot t_r \\ t_{live} =& \frac{N_{meas}}{N_p} \end{aligned} \tag{11}$$

where $t_r$ is the measurement time and $N_{meas}$ denotes the pulser peak area. The ratio $t_{live}$ is the live-time of the HPGe detector during the measurement, and is used to correct for the dead time as follows:

$$N_{\gamma-corr} = \frac{N_\gamma}{t_{live}}, \tag{12}$$

where $N_{\gamma-corr}$ is the live-time corrected number of $\gamma$-rays detected.

Since the total rate in the HPGe detector was less than 500 counts per second and the event processing time in the data acquisition is $\approx 15$ microseconds, this represents less than a 1% correction to the number of $\gamma$-rays measured. In a measurement period of 1 hour, the statistical uncertainty from the pulser measurement of the live-time is on the order of 0.02% on a 1% correction. The live-time correction contribution to the BR uncertainty is negligible.

*3.2.4. Random Coincidence*

As with $N_\beta$, among the events of 440 keV that were measured in coincidence with a $\beta$ particle, there are random coincidences. To determine the random $\beta$-$\gamma$ coincidences, the $\gamma$-ray spectrum for the coincidence 440 keV peak was determined for the prompt and random timing regions. The prompt events were found by gating on the both the scintillator (thick-thin time difference) and thick-HPGe prompt coincidence timing regions. The random background region was determined by gating on the scintillator (thick-thin time difference) coincidence window and the region outside the thick-HPGe coincidence timing region. The random spectrum was normalized (to have equal windows in the timing region) and subtracted from the prompt $\gamma$-ray spectrum. The uncertainty from this procedure was then added in to the net number of $\gamma$-rays.

*3.2.5. $N_{\beta\gamma}$ Corrections - Summary*

The term for the number of 440 keV events is written as:

$$N_{\beta\gamma} = (N^m_{\beta\gamma} \cdot N^c_{HS}) \cdot k_{thres} \cdot t^{-1}_{live}, \tag{13}$$

where $N_{\beta\gamma}$, $N^m_{\beta\gamma}$ denotes the number of 440 keV events that measured in coincidence with $\beta$ and its measured value respectively. $N_{HS}$ denote the higher state corrections, extracted from [13]. $k_{thre}$, $t_{live}$ denote the threshold and dead-time corrections.

*3.3. $\varepsilon_\gamma$ - Volume correction*

Two corrections must be applied to the measured $\gamma$-ray efficiency, both related to the extended nature of the measurement cell. Since the efficiency of the HPGe detector is measured using a point source, in order to take into account the finite measurement cell volume the $\gamma$-ray efficiency is measured

at several points on the front and back face of the measurement cell and a weighted average and associated uncertainty is calculated.

Additionally, one must consider the fact that the efficiency of detection is slightly different when detecting only $\beta$ particles or both $\beta$ and $\gamma$ particles in coincidence, due to the slightly different solid angle of the detector in both case. To account for this effect, a simulation was performed for the decay in which we compare the number of detected particles for the two cases. From the simulation, we obtain a volume correction term of $1.001 \pm 0.001$

## 4. Extraction of the branching ratio

To check the consistency between the different runs in each of the distance settings, we plot the ratio of $\beta-\gamma$ to $\beta$ events in each of the runs (note that this value is not the branching ratio, since it has not been normalized to the detector efficiency or corrected for any of the other corrections mentioned). Fig. 8 shows the ratio for all the runs. It is evident that the runs are consistent, a fact that allows us to collate all the runs for each distance summing to a single data point, which is then corrected and normalized.

We now calculate the branching ratio for each of the distance setting using Eq. (6). Fig. 9 shows the results of the calculation for both distances and the averaged value which we take to be the measured branching ratio (with the uncertainty inflated by $\sqrt{\chi^2_\nu}$).

The final value for the branching ratio to the 440-keV state is:

$$BR_{440keV} = 0.3310 \pm 0.0027 \tag{14}$$

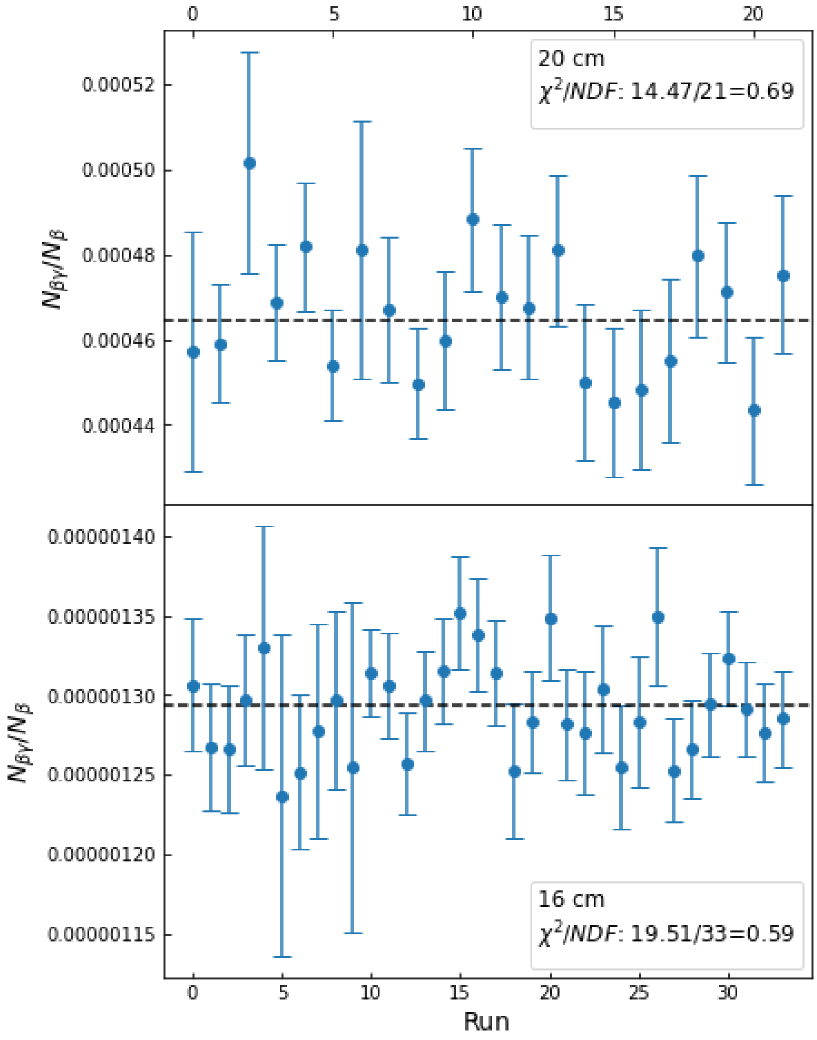


Figure 8: $N_\gamma/N_\beta$ for the individual runs (the dashed line is a fit to a constant, used to check for statistical consistency).

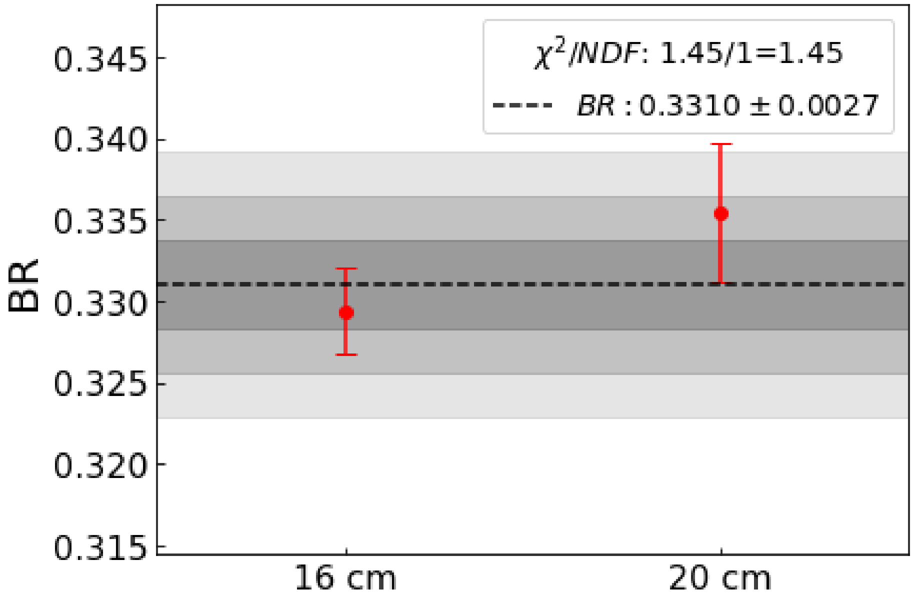


Figure 9: The measured branching ratio for the two distance settings (the bands are the $1\sigma$, $2\sigma$, and $3\sigma$ uncertainty bands.

Using our measured BR we now use the measured $\gamma$ intensity ratios from [13] to update the recommended $\beta$ transition intensities. Table 2 summarizes our recommended $\beta$ transition intensities.

| E(decay) [keV] | E(level) [keV] | I$\beta$ | Log $ft$ |
|---|---|---|---|
| (1394.0 7) | 2981.8 | 0.0675 39 | 6.13 3 |
| (2298.9 7) | 2076.9 | 1.14 6 | 5.82 2 |
| (3935.5 9) | 440.3 | 33.10 27 | 5.82 2 |
| (4375.80 10) | 0.0 | 65.69 28 | 5.27 1 |

Table 2: Recommended $\beta$ transition intensities.

Figure 10, adapted from [13] shows the decay scheme of $^{23}$Ne to $^{23}$Na, new values for the $\beta$ transition intensities are shown in red.

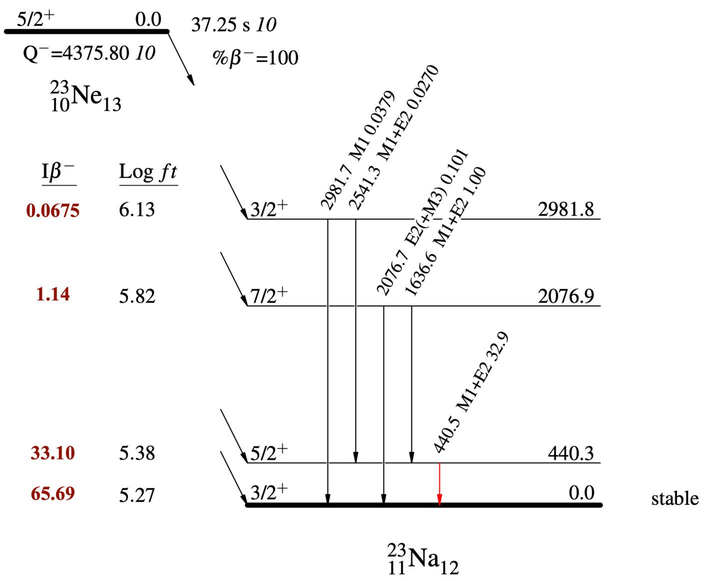


Figure 10: The $^{23}$Ne decay scheme, adapted from [13].

## 5. Validation - $^6$He

To validate the analysis method, and in particular the new theoretical calculation of the recoil order corrections, we perform the same analysis on the $^6$He data from [14], using nuclear matrix elements derived as in [15]. Since $^6$He decays exclusively to the ground state of $^6$Li via a pure Gamow-Teller decay, there are no uncertainties associated with the branching ratio. We can thus validate this analysis versus the result in [14] which is currently the best published result for $a_{\beta\nu}$. We follow the same analysis procedure outlined above, with the modification that fewer templates for the recoil ion spectra are required (since all decays are to the ground state).

Figure 11 shows the results of the fit, together with the contour plot for the joint probability density function (PDF) of $a_{\beta\nu}$ and $b_F$, the contours show the 68.3%, 95.5%, and 99.7% confidence regions.

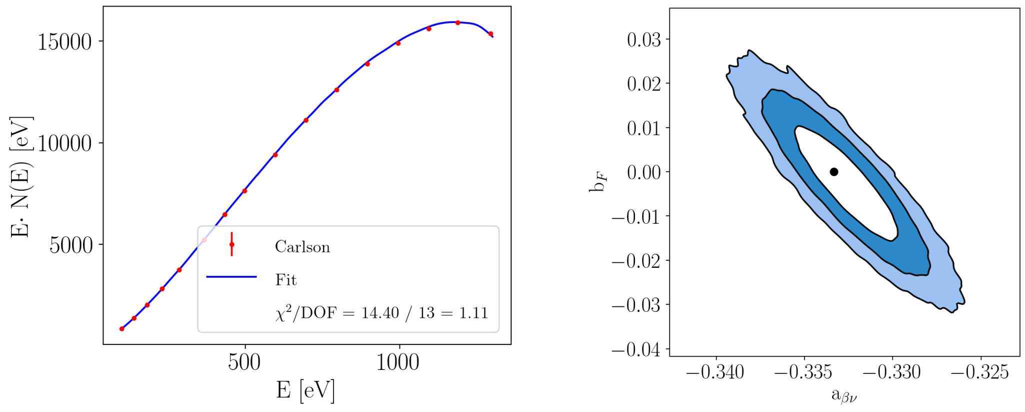


(a) (b)

Figure 11: Results of the fit to the data from [16]. (a) The fit. (b) Joint PDF for $a_{\beta\nu}$ and $b_F$, the black dot indicates the SM values.

The results of the fit give:

$$a_{\beta\nu}^{6He} = -0.3326 \pm 0.0030 \quad (15)$$

$$b_F^{6He} = -0.0026 \pm 0.0083, \quad (16)$$

in agreement with the results from [14] of:

$$a_{\beta\nu} = -0.3343 \pm 0.0030 \quad (17)$$

## 6. Explicit expressions of the multipole operators

Here we explicitly show the expressions used for the multipole operators in the recoil order correction (see Methods section in the main text).

$$\hat{L}_1^A = \frac{ig_A}{2\sqrt{3\pi}} \sum_{j=1}^{A} \vec{\sigma}_j \tau_j^+,$$
$$\frac{\hat{C}_1^A}{q} = -\frac{i}{2\sqrt{3\pi}} \frac{1}{m_N} \sum_{j=1}^{A} \left[ g_A \vec{r}_j \left( \vec{\sigma}_j \cdot \vec{\nabla}_j \right) + \frac{1}{2} \left( g_A - \frac{\tilde{g}_P}{2m_N} \left( \omega + \Delta E_c \right) \right) \vec{\sigma}_j \right] \tau_j^+,$$
$$\frac{\hat{M}_1^V}{q} = \frac{i}{2\sqrt{6\pi}} \frac{1}{m_N} \sum_{j=1}^{A} \left( g_V \vec{l}_j + \mu \vec{\sigma}_j \right) \tau_j^+, \tag{18}$$

where the $A$ above the sum symbol is the mass number of the initial- and final-state nucleus (in contrast to the superscript A(V) labeling operators calculated with the axial-vector (polar-vector) symmetry contribution to the weak nuclear current), $\vec{r}_j$ is the $j$th nucleon position vector, $\vec{l}_j$ is the nucleon angular momentum, $\tau_j^+$ is the isospin raising operator of nucleon $j$, and $\vec{\sigma}_j$ is the Pauli spin matrix associated with nucleon $j$. The vector and axial form factors are $g_V = 1$ and $g_A \approx -1.27$, the pseudoscalar form factor is $-\frac{\tilde{g}_P}{2m_N} \approx \frac{2m_N g_A}{m_\pi^2 - q^2} = \frac{2m_N g_A}{m_\pi^2} + \mathcal{O}\left(q^2\right)$ [17] (with $m_N$ the nucleon mass, and $m_\pi$ the pion mass), the isovector magnetic moment is $\mu \approx 4.706$, and $\Delta E_c$ is the Coulomb displacement energy [18] which for $^6$He is $\Delta E_c = 0.837(10)$ MeV, while for $^{23}$Ne is $\Delta E_c = 4.298(1)$ MeV [19].

## 7. Nuclear matrix elements for the $\beta$ decay of $^{23}$Ne

We calculate the leading nuclear matrix elements for the $\beta$ decay of the $5/2^+_{\rm gs}$ of $^{23}$Ne into low-lying states of $^{23}$Na, using the nuclear shell model in the sd-shell on top of a $^{16}$O core. The configuration space therefore includes the $d_{5/2}$, $s_{1/2}$ and $d_{3/2}$ single particle orbitals for neutrons and protons. We use the USDB interaction [20], which is the gold-standard shell model interaction in the sd-shell (nuclei from $^{16}$O to $^{40}$Ca), and also the USD interaction [21], a previous version of USDB built in the same spirit. We perform our calculations with the code NATHAN [22]. The calculations reproduce very well the excitation energies of the low-lying states in $^{23}$Na, with an agreement always better than 200 keV.

Since both USDB and USD interactions are isospin symmetric, all the calculated nuclear states have good isospin. For the $^{23}$Ne states isospin is T = 3/2 while for the $^{23}$Na states T = 1/2. Without isospin mixing, the Fermi operator ($\sum_j \tau_j^{\pm} = T^{\pm}$) only changes the isospin projection, leading to vanishing matrix elements between states with different isospin.

It is well known, however, that shell model matrix elements suffer from deficiencies. For instance, the Gamow-Teller matrix elements are overestimated. Nonetheless, this can be systematically fixed by correcting them by a "quenching" factor $q \approx 0.764 \pm 0.013(0.776 \pm 0.013)$ for USDB(USD) [23]. This is equivalent to using an effective value of the coupling $g_A^{\rm eff} \approx 0.970(0.986)$, and sometimes is referred to as "$g_A$ quenching". However, it is the matrix elements, and not the coupling, which need to be corrected. The underlying reason for the overestimation is a combination of missing nuclear correlations and meson-exchange currents, in comparable amount [24]. This correction needs to be applied to the GT matrix element associated with $\hat{L}_1^A$. The corresponding deficiency associated with the orbital operator $\sum_j \vec{l}_j \tau_j^+$, however, has not been explored in the literature. This term originates from the vector current, and appears together with $\sum_j \vec{\sigma}_j \tau_j^+$ (from the vector current as well). Some hints can be learned by comparing USDB(USD) results to data on the electromagnetic sector, in particular, magnetic dipole moments and transitions [23]. Focusing on the isovector part relevant for $\beta$ decay, experimental data is best reproduced with $\mu^{\rm eff} \approx 4.35 \pm 0.10(4.32 \pm 0.10)$ and $g_V^{\rm eff} \approx 1.25 \pm 0.14(1.168 \pm 0.025)$ for USDB(USD) - again, this is just a convenient way of writing: in reality the couplings are fixed, but the nuclear matrix elements are systematically overestimated (those that go with $\mu$) or underestimated (those with $g_V$). The fact that the "correction" to $g_A$ and

$\mu$, which are associated with the same Gamow- Teller operator, is different, suggests that the physics missed by the nuclear shell model in each of the two transitions is different, e.g., due to different meson exchange currents [25, 26]. Based on this, it seems appropriate to correct the shell model matrix elements for $\hat{M}_1^V$ using the factor associated with $\mu^{\rm eff}$ instead of the one corresponding to $g_A^{\rm eff}$ , used for $\hat{L}_1^A$ - this is, $\hat{M}_1^V$ is more related to electromagnetic rather than $\beta$ decays. Likewise, for the orbital transition matrix elements we should consider an enhancement of 25%(17%) in the USDB(USD) results.

These considerations result in the following nuclear matrix elements:

$$\left\langle {}^{23}\mathrm{Na}\frac{3}{2}^+_{\rm gs} \left\| \sum_j \vec{\sigma}_j \tau_j^+ \right\| {}^{23}\mathrm{Ne}\frac{5}{2}^+_{\rm gs} \right\rangle = 0.215 - 0.252,$$

$$\left\langle {}^{23}\mathrm{Na}\frac{5}{2}^+_{1} \left\| \sum_j \vec{\sigma}_j \tau_j^+ \right\| {}^{23}\mathrm{Ne}\frac{5}{2}^+_{\rm gs} \right\rangle = 0.226 - 0.265,$$

$$\left\langle {}^{23}\mathrm{Na}\frac{7}{2}^+_{1} \left\| \sum_j \vec{\sigma}_j \tau_j^+ \right\| {}^{23}\mathrm{Ne}\frac{5}{2}^+_{\rm gs} \right\rangle = 0.062 - 0.070,$$

$$\left\langle {}^{23}\mathrm{Na}\frac{3}{2}^+_{2} \left\| \sum_j \vec{\sigma}_j \tau_j^+ \right\| {}^{23}\mathrm{Ne}\frac{5}{2}^+_{\rm gs} \right\rangle = 0.165 - 0.173,$$

$$\left\langle {}^{23}\mathrm{Na}\frac{3}{2}^+_{\rm gs} \left\| \sum_j \left(\mu\vec{\sigma}_j + g_V \vec{l}_j\right) \tau_j^+ \right\| {}^{23}\mathrm{Ne}\frac{5}{2}^+_{\rm gs} \right\rangle = 4.02 - 4.78,$$

$$\left\langle {}^{23}\mathrm{Na}\frac{5}{2}^+_{1} \left\| \sum_j \left(\mu\vec{\sigma}_j + g_V \vec{l}_j\right) \tau_j^+ \right\| {}^{23}\mathrm{Ne}\frac{5}{2}^+_{\rm gs} \right\rangle = 3.40 - 4.00,$$

$$\left\langle {}^{23}\mathrm{Na}\frac{7}{2}^+_{1} \left\| \sum_j \left(\mu\vec{\sigma}_j + g_V \vec{l}_j\right) \tau_j^+ \right\| {}^{23}\mathrm{Ne}\frac{5}{2}^+_{\rm gs} \right\rangle = 1.64 - 1.96,$$

$$\left\langle {}^{23}\mathrm{Na}\frac{3}{2}^+_{2} \left\| \sum_j \left(\mu\vec{\sigma}_j + g_V \vec{l}_j\right) \tau_j^+ \right\| {}^{23}\mathrm{Ne}\frac{5}{2}^+_{\rm gs} \right\rangle = 0.99 - 1.05,$$

which have uncertainties of about 10% from the different interactions used (on the amplitudes, so twice as much on observables). The main point from the nuclear structure side is that GT matrix elements are 15-20 times smaller than magnetic ones, which is somewhat larger than the expected factor $\mu/g_A \sim 4$ due to the orbital angular momentum contributions.

[1] S. Halfon, A. Arenshtam, D. Kijel, M. Paul, D. Berkovits, I. Eliyahu, G. Feinberg, M. Friedman, N. Hazenshprung, I. Mardor, et al., High-power liquid-lithium jet target for neutron production, Review of scientific instruments 84 (12) (2013) 123507.

[2] S. Halfon, A. Arenshtam, D. Kijel, M. Paul, L. Weissman, O. Aviv, D. Berkovits, O. Dudovitch, Y. Eisen, I. Eliyahu, et al., Note: Proton irradiation at kilowatt-power and neutron production from a free-surface liquid-lithium target, Review of Scientific Instruments 85 (5) (2014) 056105.

[3] S. Halfon, A. Arenshtam, D. Kijel, M. Paul, L. Weissman, D. Berkovits, I. Eliyahu, G. Feinberg, A. Kreisel, I. Mardor, et al., Demonstration of a high-intensity neutron source based on a liquid-lithium target for accelerator based boron neutron capture therapy, Applied Radiation and Isotopes 106 (2015) 57–62.

[4] M. Paul, A. Arenshtam, S. Halfon, D. Kijel, M. Tessler, L. Weissman, D. Berkovits, Y. Eisen, I. Eliyahu, M. Friedman, et al., A high-power liquid-lithium target (lilit) for neutron production, Journal of Radioanalytical and Nuclear Chemistry 305 (3) (2015) 783–786.

[5] M. Paul, M. Tessler, M. Friedman, S. Halfon, T. Palchan, L. Weissman, A. Arenshtam, D. Berkovits, Y. Eisen, I. Eliahu, G. Feinberg, D. Kijel, A. Kreisel, I. Mardor, G. Shimel, A. Shor, I. Silverman, Reactions along the astrophysical s-process path and prospects for neutron radiotherapy with the Liquid-Lithium Target (LiLiT) at the Soreq Applied Research Accelerator Facility (SARAF), European Physical Journal A 55 (3) (2019) 44. doi:10.1140/epja/i2019-12723-5.

[6] Y. Mishnayot, H. Rahangdale, B. Ohayon, S. Vaintraub, T. Hirsh, L. Weismann, A. Perry, A. Shor, A. Kreisel, S. Ya'akobi, E. Buznach, G. Ron, $^{23}$ne production at saraf-i, Nuclear Instruments and Methods in Physics Research Section A: Accelerators, Spectrometers, Detectors and Associated Equipment 978 (2020) 164365. doi:https://doi.org/10.1016/j.nima.2020.164365.
URL https://www.sciencedirect.com/science/article/pii/S0168900220307622

[7] M. J. Safari, F. A. Davani, H. Afarideh, Differentiation method for localization of Compton edge in organic scintillation detectorsarXiv:1610.09185.

[8] G. F. Knoll, Radiation detection and measurement, John Wiley & Sons, 2010.

[9] S. Agostinelli, J. Allison, K. Amako, J. Apostolakis, H. Araujo, P. Arce, M. Asai, D. Axen, S. Banerjee, G. Barrand, F. Behner, L. Bellagamba, J. Boudreau, L. Broglia, A. Brunengo, H. Burkhardt, S. Chauvie, J. Chuma, R. Chytracek, G. Cooperman, G. Cosmo, P. Degtyarenko, A. Dell'Acqua, G. Depaola, D. Dietrich, R. Enami, A. Feliciello, C. Ferguson, H. Fesefeldt, G. Folger, F. Foppiano, A. Forti, S. Garelli, S. Giani, R. Giannitrapani, D. Gibin, J. G. Cadenas], I. González, G. G. Abril], G. Greeniaus, W. Greiner, V. Grichine, A. Grossheim, S. Guatelli, P. Gumplinger, R. Hamatsu, K. Hashimoto, H. Hasui, A. Heikkinen, A. Howard, V. Ivanchenko, A. Johnson, F. Jones, J. Kallenbach, N. Kanaya, M. Kawabata, Y. Kawabata, M. Kawaguti, S. Kelner, P. Kent, A. Kimura, T. Kodama, R. Kokoulin, M. Kossov, H. Kurashige, E. Lamanna, T. Lampén, V. Lara, V. Lefebure, F. Lei, M. Liendl, W. Lockman, F. Longo, S. Magni, M. Maire, E. Medernach, K. Minamimoto, P. M. de Freitas], Y. Morita, K. Murakami, M. Nagamatu, R. Nartallo, P. Nieminen, T. Nishimura, K. Ohtsubo, M. Okamura, S. O'Neale, Y. Oohata, K. Paech, J. Perl, A. Pfeiffer, M. Pia, F. Ranjard, A. Rybin, S. Sadilov, E. D. Salvo], G. Santin, T. Sasaki, N. Savvas, Y. Sawada, S. Scherer, S. Sei, V. Sirotenko, D. Smith, N. Starkov, H. Stoecker, J. Sulkimo, M. Takahata, S. Tanaka, E. Tcherniaev, E. S. Tehrani], M. Tropeano, P. Truscott, H. Uno, L. Urban, P. Urban, M. Verderi, A. Walkden, W. Wander, H. Weber, J. Wellisch, T. Wenaus, D. Williams, D. Wright, T. Yamada, H. Yoshida, D. Zschiesche, Geant4—a simulation toolkit, Nuclear Instruments and Methods in Physics Research Section A: Accelerators, Spectrometers, Detectors and Associated Equipment 506 (3) (2003) 250 – 303. doi:https://doi.org/10.1016/S0168-9002(03)01368-8. URL http://www.sciencedirect.com/science/article/pii/S0168900203013688

[10] J. Allison, K. Amako, J. Apostolakis, H. Araujo, P. Arce Dubois, M. Asai, G. Barrand, R. Capra, S. Chauvie, R. Chytracek, G. A. P.

Cirrone, G. Cooperman, G. Cosmo, G. Cuttone, G. G. Daquino, M. Donszelmann, M. Dressel, G. Folger, F. Foppiano, J. Generowicz, V. Grichine, S. Guatelli, P. Gumplinger, A. Heikkinen, I. Hrivnacova, A. Howard, S. Incerti, V. Ivanchenko, T. Johnson, F. Jones, T. Koi, R. Kokoulin, M. Kossov, H. Kurashige, V. Lara, S. Larsson, F. Lei, O. Link, F. Longo, M. Maire, A. Mantero, B. Mascialino, I. McLaren, P. Mendez Lorenzo, K. Minamimoto, K. Murakami, P. Nieminen, L. Pandola, S. Parlati, L. Peralta, J. Perl, A. Pfeiffer, M. G. Pia, A. Ribon, P. Rodrigues, G. Russo, S. Sadilov, G. Santin, T. Sasaki, D. Smith, N. Starkov, S. Tanaka, E. Tcherniaev, B. Tome, A. Trindade, P. Truscott, L. Urban, M. Verderi, A. Walkden, J. P. Wellisch, D. C. Williams, D. Wright, H. Yoshida, Geant4 developments and applications, IEEE Transactions on Nuclear Science 53 (1) (2006) 270–278.

[11] J. Allison, K. Amako, J. Apostolakis, P. Arce, M. Asai, T. Aso, E. Bagli, A. Bagulya, S. Banerjee, G. Barrand, B. Beck, A. Bogdanov, D. Brandt, J. Brown, H. Burkhardt, P. Canal, D. Cano-Ott, S. Chauvie, K. Cho, G. Cirrone, G. Cooperman, M. Cortés-Giraldo, G. Cosmo, G. Cuttone, G. Depaola, L. Desorgher, X. Dong, A. Dotti, V. Elvira, G. Folger, Z. Francis, A. Galoyan, L. Garnier, M. Gayer, K. Genser, V. Grichine, S. Guatelli, P. Guèye, P. Gumplinger, A. Howard, I. Hřivnáčová, S. Hwang, S. Incerti, A. Ivanchenko, V. Ivanchenko, F. Jones, S. Jun, P. Kaitaniemi, N. Karakatsanis, M. Karamitros, M. Kelsey, A. Kimura, T. Koi, H. Kurashige, A. Lechner, S. Lee, F. Longo, M. Maire, D. Mancusi, A. Mantero, E. Mendoza, B. Morgan, K. Murakami, T. Nikitina, L. Pandola, P. Paprocki, J. Perl, I. Petrović, M. Pia, W. Pokorski, J. Quesada, M. Raine, M. Reis, A. Ribon, A. R. Fira], F. Romano, G. Russo, G. Santin, T. Sasaki, D. Sawkey, J. Shin, I. Strakovsky, A. Taborda, S. Tanaka, B. Tomé, T. Toshito, H. Tran, P. Truscott, L. Urban, V. Uzhinsky, J. Verbeke, M. Verderi, B. Wendt, H. Wenzel, D. Wright, D. Wright, T. Yamashita, J. Yarba, H. Yoshida, Recent developments in geant4, Nuclear Instruments and Methods in Physics Research Section A: Accelerators, Spectrometers, Detectors and Associated Equipment 835 (2016) 186 – 225. doi:https://doi.org/10.1016/j.nima.2016.06.125.
URL http://www.sciencedirect.com/science/article/pii/S0168900216306957

[12] L. Hayen, N. Severijns, Beta spectrum generator: High precision allowed $\beta$ spectrum shapes, Computer Physics Communications 240 (2019) 152–164.

[13] M. Shamsuzzoha Basunia, A. Chakraborty, Nuclear data sheets for a=23, Nuclear Data Sheets 171 (2021) 1–252. doi:https://doi.org/10.1016/j.nds.2020.12.001.
URL https://www.sciencedirect.com/science/article/pii/S0090375220300582

[14] C. H. Johnson, F. Pleasonton, T. A. Carlson, Precision Measurement of the Recoil Energy Spectrum from the Decay of $He^6$, Physical Review 132 (3) (1963) 1149–1165. doi:10.1103/PhysRev.132.1149.

[15] A. Glick-Magid, C. Forssén, D. Gazda, D. Gazit, P. Gysbers, P. Navrátil, Nuclear ab initio calculations of $^6$he $\beta$-decay for beyond the standard model studies (2021). arXiv:2107.10212.

[16] T. A. Carlson, Recoil energy spectrum of the sodium ions following the $\beta^-$ decay of $ne^{23}$, Phys. Rev. 132 (1963) 2239–2242. doi:10.1103/PhysRev.132.2239.
URL https://link.aps.org/doi/10.1103/PhysRev.132.2239

[17] J. Walecka, Section 4 - semileptonic weak interactions in nuclei**research sponsored by the air force office of scientific research, office of aerospace research, u.s. air force, under afosr contract no. f44620-71-c-0044., in: V. W. Hughes, C. Wu (Eds.), Muon Physics, Academic Press, 1975, pp. 113–218. doi:https://doi.org/10.1016/B978-0-12-360602-0.50010-5.
URL https://www.sciencedirect.com/science/article/pii/B9780123606020500105

[18] H. Behrens, W. Bühring, Electron radial wave functions and nuclear beta-decay, no. 67, Oxford University Press, USA, 1982.

[19] M. Antony, A. Pape, J. Britz, Coulomb displacement energies between analog levels for $3 \leq a \leq 239$, Atomic Data and Nuclear Data Tables 66 (1) (1997) 1–63. doi:https://doi.org/10.1006/adnd.1997.0740.
URL https://www.sciencedirect.com/science/article/pii/S0092640X97907403

[20] B. A. Brown, W. Richter, New “usd” hamiltonians for the sd shell, Physical Review C 74 (3) (2006) 034315.

[21] B. Wildenthal, Empirical strengths of spin operators in nuclei, Progress in particle and nuclear physics 11 (1984) 5–51.

[22] E. Caurier, G. Martinez-Pinedo, F. Nowacki, A. Poves, A. Zuker, The shell model as a unified view of nuclear structure, Reviews of Modern Physics 77 (2) (2005) 427.

[23] W. Richter, S. Mkhize, B. A. Brown, sd-shell observables for the usda and usdb hamiltonians, Physical Review C 78 (6) (2008) 064302.

[24] P. Gysbers, G. Hagen, J. Holt, G. R. Jansen, T. D. Morris, P. Navrátil, T. Papenbrock, S. Quaglioni, A. Schwenk, S. Stroberg, et al., Discrepancy between experimental and theoretical $\beta$-decay rates resolved from first principles, Nature Physics 15 (5) (2019) 428–431.

[25] H. Krebs, E. Epelbaum, U.-G. Meißner, Nuclear axial current operators to fourth order in chiral effective field theory, Annals of physics 378 (2017) 317–395.

[26] S. Bacca, S. Pastore, Electromagnetic reactions on light nuclei, Journal of Physics G: Nuclear and Particle Physics 41 (12) (2014) 123002.
